# Supplementary material for: Embedded Index Coding
Source: arXiv:1904.02179 source file (2019-10-30)
Supplement: Supplementary file 1 [file appendix.tex]

% !TEX root = distribIC_ITW19.tex
\subsection{Extended Related Work}
Linear, centralized, non-cooperative approaches to index coding include maximum acyclic induced subgraph and rank over digraph-induced matrices~\cite{bar2006index}, cycle-covering~\cite{chaudhry2011complementary}, local chromatic number~\cite{shanmugam2013local} and interlinked cycle covering~\cite{thapa2017interlinked}.
%\TODO{check these are centralized, maybe if scalar or vector: original is just bits from single source, complementary is scalar+vector decentralized,  local graph coloring is general (i.e. vector) and centralized, }

Linear index coding can be \emph{scalar} or \emph{vector}~\cite{chaudhry2011complementary}: scalar-linear solutions allow do not allow packet splitting while vector-linear solutions do.

\begin{itemize}
\item Algorithms~\cite{chaudhry2008efficient}: Chaudhry et al. give a reduction from the index coding problem to a SAT problem and show that a SAT solver gives the optimal solution. They also show that the optimal index coding solution can be approximated with heuristics from graph coloring, sparseset set clustering, and a color saving heuristic. The coloring approach corresponds to a known upper bound on index coding, the complement coloring upper bound on the minrank of a graph. %Our $e_j$ being the indicator vector is the same as that position in the vector in the algorithms paper being 1 if the block is had or needed, but then~\cite{chaudhry2008efficient} entries that would be in $\beta,\alpha$ as in GF(2); also the goal is decode one packet each in a fixed number of messages, not doing any minimization.

\item Complementary Index Coding~\cite{chaudhry2011complementary,neely2013dynamic}: While the index coding problem has shown to be NP-Hard, Chaudhry et al. introduce the  \emph{Complementary Index Coding} problem, in which the goal is to maximize the number of saved transmissions (i.e. compared to a simple or naive solution) rather than minimize the total transmission. This complementary problem allows for new approximations. In~\cite{neely2013dynamic}, coding actions able to improve over uncoded transmission are described, and it is shown that cycle exploitation is sufficient for an optimal algorithm in a class of problems.

\item Critical Graphs~\cite{tahmasbi2015critical}: In~\cite{tahmasbi2015critical}, it is shown that for linear index codes, a union of strongly connected subgraphs (USCS) is the critical subgraph of a side information graph, meaning removal of edges not included in the USCS does not change the rate region to which the graph corresponds.

\item Extending to two senders~\cite{thapa2016graph}: It was shown by~\cite{thapa2016graph} that in some cases, two-sender unicast index codes are equivalent to single sender index codes, and single-sender schemes including clique-cover were extended to two-sender. As in single-sender clique cover, a coded symbol can be produced and transmitted for each clique such that all vertices in the clique can decode their requested message; however there is an additional constraint that one of the two senders has all of the requested blocks so that it can produce such a symbol.

\item Storage Duality~\cite{mazumdar2014duality}: The relationship between an optimal recoverable distributed storage code and an optimal index code (general, not linear) is shown by~\cite{mazumdar2014duality}, by using a graph $G$ as both a distributed storage graph and a side information graph.

\item LRC Duality~\cite{shanmugam2014bounding}: Linear index codes were shown by~\cite{shanmugam2014bounding} to be dual to an extension of LRCs, Generalized Locally Repairable Codes. In the GLRC, a graph specifies the recoverability set from which each node is decodable; this graph servers as the side information graph in an index coding instance. Then the redundancy of the index code, or the complementary index coding rate (\cite{chaudhry2011complementary}), is the rate of the GLRC. Results are generalized by~\cite{arbabjolfaei2015three} to show that the capacity and optimal rates of the index coding and LRC problems are complementary.

\item Multiple requests~\cite{lubetzky2009nonlinear}: shows that the minrank tightness extends to when multiple nodes may request the same block (but each node still requesting one).

\item Non-Linear~\cite{lubetzky2009nonlinear}: It has also been established that non-linear index coding out-performs linear index codes for some sufficiently large side-information graphs.

\item Instantly decodable~\cite{le2013instantly}: Instantly Decodable Network Codes (IDNC's) minimize completion delay, the time it takes for nodes to all recover lost information. Real-Time IDNC, introduced by~\cite{le2013instantly}, aims to choose coded packets to be broadcast from the source such that the maximum number of users can immediately recover a lost packet from a single broadcast; they show this problem is equivalent to maximum clique on the corresponding graph (also same as strongly task based).

\item Limitations of graph-theoretic bounds~\cite{blasiak2013broadcasting,shanmugam2014graph}: The upper and lower bounds of minrank of a side information graph, and thus the broadcast rate of an index code, based on coloring and independent set have been shown to have substantial gaps in some settings. In~\cite{} there is a separation between the $\alpha(G)$ lower bound and the index code rate established which goes to infinity for a sequence of graphs. The coloring of the complement graph, $\overline{\chi}$, and the improved upper bound of the fractional clique cover $\overline{\chi}_f \leq \overline{\chi})$, are also shown to be  potentially unbounded by any function of the code rate. Then~\cite{shanmugam2014graph} shows that graph theoretic bounds in general not much stronger than the chromatic number upper bound.

\end{itemize}
\subsection{Random Decentralized Index Coding}

The line of work beginning with~\cite{sadeghi2016distributed} and continued in~\cite{li2017improved,li2018cooperative} explores multi-sender models for index coding and specifies achievable rate regions using \emph{composite coding}, first introduced in the centralized setting~\cite{arbabjolfaei2013capacity} based on randomized coding. While our coding scheme is deterministic and linear, our network model is similar to these.

Introduced by~\cite{sadeghi2016distributed}, Distributed Composite Coding (DCC) assumes there exists a sender with each possible combination of data blocks. Receivers are then a separate set of nodes, each of which is requesting exactly one unique block (so there are as many blocks as receivers). The model also specifies a broadcast link capacity between each sender and the full set of receivers; achievable rate regions are established given the link capacities. DCC partitions senders into non-overlapping groups, with messages appearing more than once split up. Composite coding is then solved independently for each group. 

Then~\cite{li2018cooperative} introduced an improvement with Cooperative Composite Coding, which allows senders to split their link capacity to participate in multiple sender groups. The model is a slight variation, in which there is a fixed number of senders $K$ and non-zero broadcast link capacity available from each sender. This can be considered a case of the DCC model, since in DCC an equivalent subset of the senders may be the only ones with non-zero broadcast capacity. The limitations of DCC addressed by CCC include the fact that senders treat the data they are broadcasting as unique from other senders, even if the same block may be repeated in different sender groups,  and the fact that each sender uses their entire link capacity participating in at most a single sender group. The first issue is addressed by \emph{cooperative compression}, which allows senders to work together if they share a combination of messages. The second is addressed by \emph{joint link-and-sender} partitioning, which allows each sender to split their bandwidth among participating in multiple sender groups. Our scheme is conceptually closest to $\mathcal{R}_C$ in~\cite{li2018cooperative}, in which all senders are a single group and composite message compression is used. 
%The improvement of joint partitioning was also used in the mDCC~\cite{li2017improved} model, but without cooperative compression. Fractional Distributed Composite coding~\cite{liu2017capacity} also applies an enhanced composite coding to fractional partitions of the servers.

\subsection{Linear Decentralized Index Coding}

Very recently,~\cite{kim2019linear} introduced a general linear model in which multiple blocks may be requested, senders have fixed sets of blocks, and encoding is linear without limitations on capacity. The minrank solution of their matrix is very similar to our solution for decentralized in general; however we show that in the case of senders being receivers only twice the minrank of a matrix of order up to $n$ is necessary, as opposed to the minrank of an order-$n^2$ matrix (with some other constraints) constructed for the problem in~\cite{kim2019linear}.

In~\cite{li2018multi} the problem of multi-sender index coding is also studied, and framed in terms of rank minimization. In their model, there are $N$ messages, each requested by exactly one unique receiver. There are $K$ senders, each with a subset of the $N$ messages available. The problem is framed as finding the lowest-ranking matrix $C$, composed of submatrices which correspond to senders, such that each request can be satisfied by $C$ as a whole. They further show that this is equivalent to solving the problem without weak senders (those with only a subset of a single other node's information), with the submatrices restricted to being lower-triangular, and redundant rows between sender submatrices removed. They give the Combined LT-CMAR process for finding a matrix $\overline{C}''$ containing $0$'s and unknown entries; this process also produces an ordering on data blocks which is then used in their algorithm to approximate the lowest ranking matrix that fits the constraints given by $\overline{C}''$ and allows all requests to be satisfied (i.e., $0$ where $\overline{C}''$ is $0$ and $0$ or $1$ at unspecified entries, and all receivers can decode their data block).

\subsection{Coded Caching}
Coded Caching is also closely related. Generally, the goal is to use coding in local caches and in transmission signals to reduce communication load. While the delivery mechanism, using coded transmissions and locally available information, can be thought of as an instance of index coding, the choice in cache contents makes the problem being solved different. 
Recent bounds on the achievable rate of coded caching, i.e. the minimum necessary transmission rate, are given in ~\cite{ghasemi2017improved}. Additionally, work has been done on decentralized coded caching, optimizing the memory-rate trade-off~\cite{maddah2015decentralized}. They give an algorithm for constructed coded broadcast messages which considers all possible groups of receivers, in descending order, and sends the sums of blocks known by all in the group except the node that needs them, i.e. the maximal strong task for the group if it exists.
